# Supplementary material for: Analytical model and experimental validation for nonlinear mechanical response of aspirated elastic shells
Source: arXiv:2504.21283 source file (2025-04-30)
Supplement: Supplementary file 1 [file SI_masuda_rev.pdf]

**Supplemental Materials for**

**Analytical model and experimental validation for nonlinear  
mechanical response of aspirated elastic shells**

Kazutoshi Masuda<sup>1</sup> and Miho Yanagisawa<sup>1,2,3,4\*</sup>

<sup>1</sup>Department of Basic Science, Graduate School of Arts and Sciences, The University of Tokyo, Komaba 3-8-1, Meguro, Tokyo 153-8902, Japan

<sup>2</sup>Komaba Institute for Science, Graduate School of Arts and Sciences, The University of Tokyo, Komaba 3-8-1, Meguro, Tokyo 153-8902, Japan

<sup>3</sup>Center for Complex Systems Biology, Universal Biology Institute, The University of Tokyo, Komaba 3-8-1, Meguro, Tokyo 153-8902, Japan

<sup>4</sup>Department of Physics, Graduate School of Science, The University of Tokyo, Hongo 7-3-1, Bunkyo, Tokyo 113-0033, Japan

Corresponding Authors

(K. M.) [kazumassuu@g.ecc.u-tokyo.ac.jp](mailto:kazumassuu@g.ecc.u-tokyo.ac.jp)

(M. Y.) [myanagisawa@g.ecc.u-tokyo.ac.jp](mailto:myanagisawa@g.ecc.u-tokyo.ac.jp)

### S1. DNA Oligonucleotides.

DNA oligonucleotides were designed based on previous research [1].

Y0-1 CAGTGAGGACGGAAGTTTGTCTAGCATCGCACC

Y0-2 CAACCACGCCTGTCCATTACTTCCGTCCTCACTG

Y0-3 GGTGCGATGCTACGACTTTGGACAGGCGTGTTG

Y4-1 GCGCCAGTGAGGACGGAAGTTTGTCTAGCATCGCACC

Y4-2 GCGCCAACCACGCCTGTCCATTACTTCCGTCCTCACTG

Y4-3 GCGCGGTGCGATGCTACGACTTTGGACAGGCGTGTTG

**S2. DNA Self-assembly in droplets.** DNA oligomers were dissolved in buffer (20 mM Tris-HCl, pH 8.0, and 350 mM NaCl) to a final concentration of 5 mM at room temperature ( $\sim 20^\circ\text{C}$ ). The solution was heated at  $80^\circ\text{C}$  for 10 minutes and then gradually cooled to  $20^\circ\text{C}$  at a rate of  $0.005^\circ\text{C/s}$  using a thermal cycler to promote hybridization. Microdroplets were prepared using a previously reported method [1]. Briefly, dry lipid films were formed at the bottom of a glass tube, dissolved in hexadecane to a final concentration of 1 mM, and subjected to ultrasonication for 90 minutes. Lipid-coated droplets were generated by mixing the hybridized DNA solution with the lipid-in-oil mixture at a 1:20 volume ratio and dispersing the mixture by pipetting.

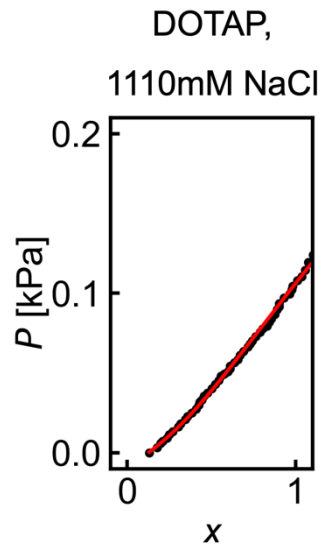

FIG. 1. An example of measured data and their fitting for a DOTAP droplet with 1110 mM NaCl, three times higher than the others, indicates a downward-convex relationship between aspiration pressure and deformation.

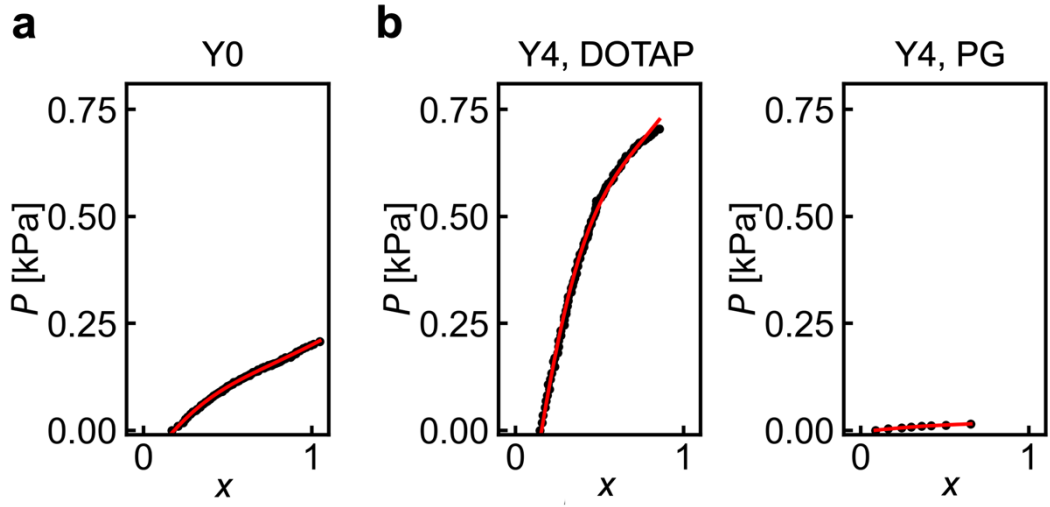

FIG. 2. Examples of measured data aspirated by a pipette with  $R_p=12\ \mu\text{m}$  and their fittings for (a) Y0 in a DOTAP droplet and (b) Y4 within a DOTAP (left) and a PG droplet (right). Since both PG and DNA gels are negatively charged, Y4 within a PG droplet is assumed not to localize underneath the PG membrane due to electrostatic repulsion, showing lower  $P$  with the same deformation as Y4 within a DOTAP droplet.

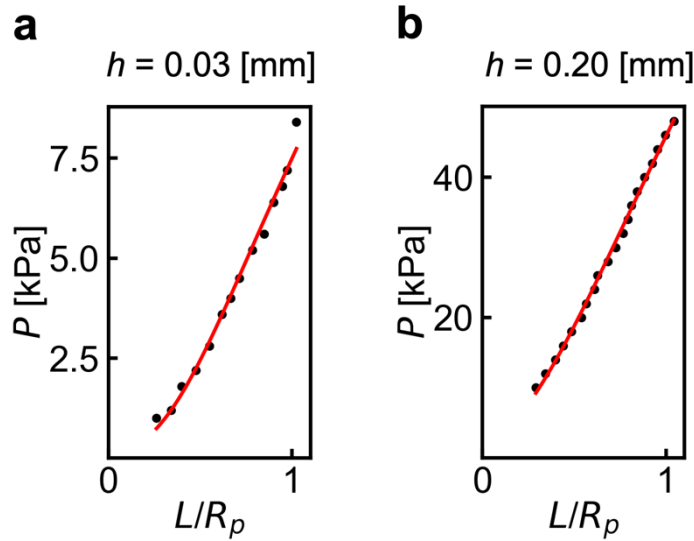

FIG. 3. Examples of measured data deformed by a desiccator  $R_p=11.5\ \text{mm}$  and their fittings for silicone sheets with different thicknesses; (a)  $h = 0.03\ \text{mm}$  and (b)  $h = 0.20\ \text{mm}$ .

## Reference

- [1] C. Kurokawa, K. Fujiwara, M. Morita, I. Kawamata, Y. Kawagishi, A. Sakai, Y. Murayama, S. I. M. Nomura, S. Murata, M. Takinoue, and M. Yanagisawa, Dna cytoskeleton for stabilizing artificial

cells, *Proceedings of the National Academy of Sciences of the United States of America* 114, 7228 (2017).
